# Supplementary material for: New allometric models for the USA create a step-change in forest carbon estimation, modeling, and mapping
Source: arXiv:2405.04507 ancillary file (2024-05-07)
Supplement: Supplementary file 1 [file supplements.pdf]

# Supplements

## Table of contents

Supplementary Materials A: Model test set accuracy . . . . . . . . . . . . . . . . . . . . . 2
Supplementary Materials B: Rescaling CRM AGB to NSVB AGB . . . . . . . . . . . 3

## Supplementary Materials A: Model test set accuracy

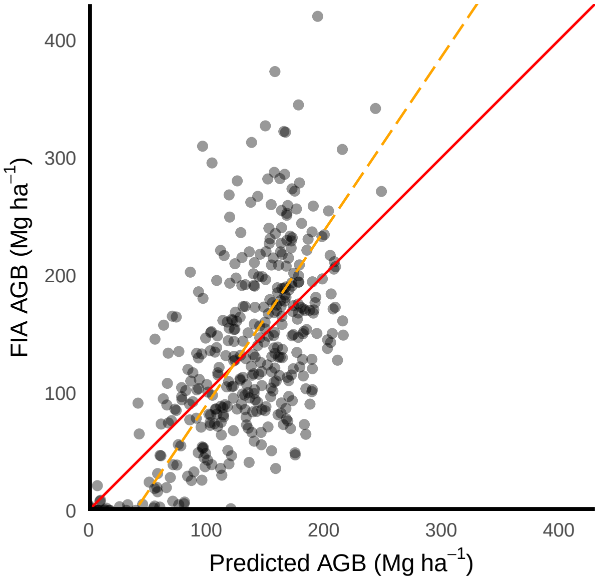


Figure 1: Comparison of predicted AGB to FIA AGB for 20%. partition of the model testing set. Geometric mean functional relationship (GMFR) trend line shown with dashed (orange) line, and 1:1 line shown with solid (red) line.

Table 1: Model performance metrics (as defined in Section 2.3) against 20% testing partition of the model development dataset.

| MAE | % MAE | RMSE | % RMSE | ME | $R^2$ |
|---|---|---|---|---|---|
| 45.04 | 35.31 | 59.29 | 46.48 | 1.72 | 0.47 |

## Supplementary Materials B: Rescaling CRM AGB to NSVB AGB

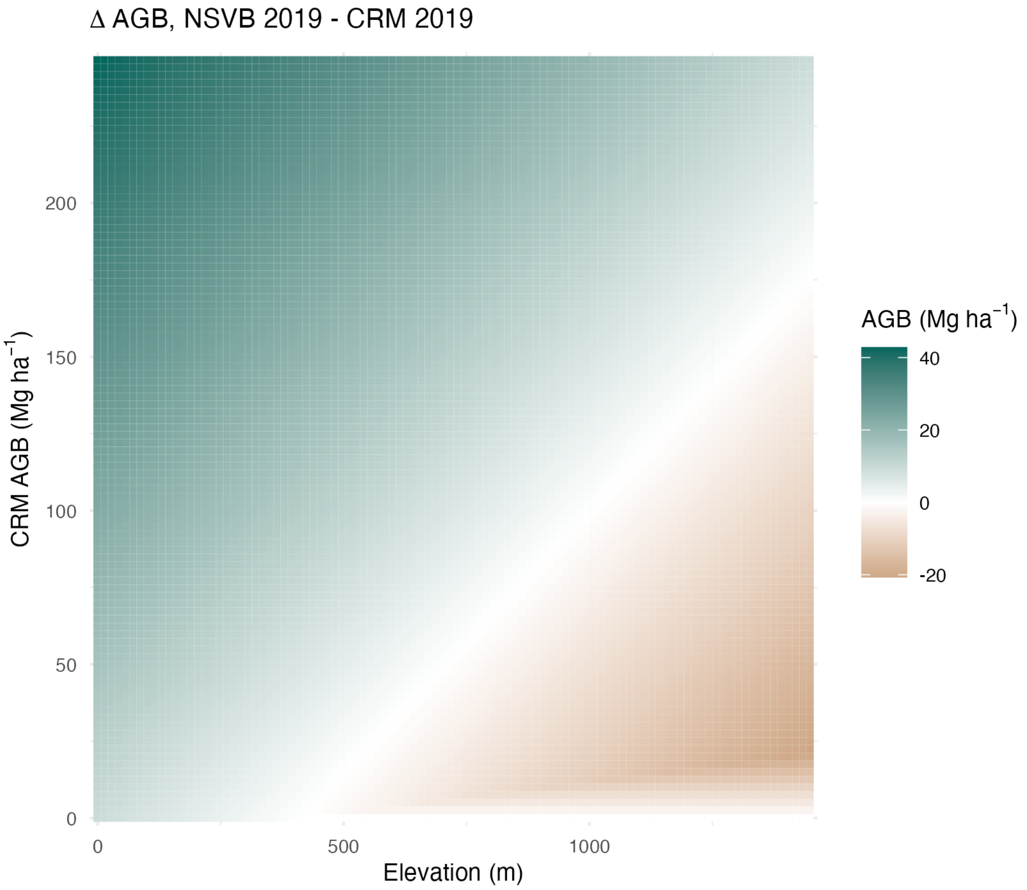


Figure 2: Heatmap describing shifts from model-based CRM AGB to model-based NSVB AGB based on predictions from a regression model that represents model-based NSVB AGB (Mgha$^{-1}$) as a function of model-based CRM AGB (Mgha$^{-1}$) and elevation (m).
